# Supplementary material for: Shape-aware Text-driven Layered Video Editing
Source: arXiv:2301.13173 source file (2023-01-30)
Supplement: Supplementary file 1 [file fig_supp_additional_visual_results.tex]

\begin{figure*}[h]
    \centering
    \frame{\includegraphics[width=0.245\linewidth]{figures/additional_visual/swan/input/00010.png}}
    \frame{\includegraphics[width=0.245\linewidth]{figures/additional_visual/swan/input/00020.png}}
    \frame{\includegraphics[width=0.245\linewidth]{figures/additional_visual/swan/input/00030.png}}
    \frame{\includegraphics[width=0.245\linewidth]{figures/additional_visual/swan/input/00040.png}} \\
    \vspace{0.1cm}
    \frame{\includegraphics[width=0.245\linewidth]{figures/additional_visual/swan/output/00010.png}}
    \frame{\includegraphics[width=0.245\linewidth]{figures/additional_visual/swan/output/00020.png}}
    \frame{\includegraphics[width=0.245\linewidth]{figures/additional_visual/swan/output/00030.png}}
    \frame{\includegraphics[width=0.245\linewidth]{figures/additional_visual/swan/output/00040.png}} \\
    ``\texttt{black swan}~\textrightarrow~\texttt{white swan}'' + ``\texttt{river}~\textrightarrow~\texttt{cartoon-style river}'' \\
    \vspace{0.3cm}
    \frame{\includegraphics[width=0.245\linewidth]{figures/additional_visual/surf/input/00005.png}}
    \frame{\includegraphics[width=0.245\linewidth]{figures/additional_visual/surf/input/00015.png}}
    \frame{\includegraphics[width=0.245\linewidth]{figures/additional_visual/surf/input/00025.png}}
    \frame{\includegraphics[width=0.245\linewidth]{figures/additional_visual/surf/input/00035.png}} \\
    \vspace{0.1cm}
    \frame{\includegraphics[width=0.245\linewidth]{figures/additional_visual/surf/output/00005.png}}
    \frame{\includegraphics[width=0.245\linewidth]{figures/additional_visual/surf/output/00015.png}}
    \frame{\includegraphics[width=0.245\linewidth]{figures/additional_visual/surf/output/00025.png}}
    \frame{\includegraphics[width=0.245\linewidth]{figures/additional_visual/surf/output/00035.png}} \\
    ``\texttt{surfing}~\textrightarrow~\texttt{sail boat}'' + ``\texttt{sea}~\textrightarrow~\texttt{cartoon-style sea with strong wave}'' \\
    \caption{\textbf{Additional visual results with foreground and background editing.}}
    \label{fig:supp_visual_results}
\end{figure*}
