# Supplementary material for: Shape-aware Text-driven Layered Video Editing
Source: arXiv:2301.13173 source file (2023-01-30)
Supplement: Supplementary file 2 [file fig_supp_edit_bg_atlas.tex]

\begin{figure}
    \centering
    \mpage{0.02}{\raisebox{2cm}{\rotatebox{90}{\hspace{0.4cm}Atlas}}}
    \frame{\includegraphics[width=0.23\linewidth]{figures/edit_atlas/bg_input/atlas.png}}
    \frame{\includegraphics[width=0.23\linewidth]{figures/edit_atlas/bg_example1/atlas.png}}
    \frame{\includegraphics[width=0.23\linewidth]{figures/edit_atlas/bg_example2/atlas.png}}
    \frame{\includegraphics[width=0.23\linewidth]{figures/edit_atlas/bg_example3/atlas.png}} \\
    \vspace{-1.38cm}
    \hline
    \vspace{0.1cm}
    \mpage{0.02}{\raisebox{2cm}{\rotatebox{90}{$\longleftarrow$ time}}}
    \frame{\includegraphics[width=0.23\linewidth]{figures/edit_atlas/fg_input/00025.png}}
    \frame{\includegraphics[width=0.23\linewidth]{figures/edit_atlas/bg_example1/00025.png}}
    \frame{\includegraphics[width=0.23\linewidth]{figures/edit_atlas/bg_example2/00025.png}}
    \frame{\includegraphics[width=0.23\linewidth]{figures/edit_atlas/bg_example3/00025.png}} \\
    \vspace{-1.5cm}
    \mpage{0.02}{\raisebox{2cm}{\rotatebox{90}{}}}
    \frame{\includegraphics[width=0.23\linewidth]{figures/edit_atlas/fg_input/00040.png}}
    \frame{\includegraphics[width=0.23\linewidth]{figures/edit_atlas/bg_example1/00040.png}}
    \frame{\includegraphics[width=0.23\linewidth]{figures/edit_atlas/bg_example2/00040.png}}
    \frame{\includegraphics[width=0.23\linewidth]{figures/edit_atlas/bg_example3/00040.png}} \\
    \vspace{-0.85cm}
    \mpage{0.02}{\raisebox{2cm}{\rotatebox{90}{}}}
    \frame{\includegraphics[width=0.23\linewidth]{figures/edit_atlas/fg_input/00055.png}}
    \frame{\includegraphics[width=0.23\linewidth]{figures/edit_atlas/bg_example1/00055.png}}
    \frame{\includegraphics[width=0.23\linewidth]{figures/edit_atlas/bg_example2/00055.png}}
    \frame{\includegraphics[width=0.23\linewidth]{figures/edit_atlas/bg_example3/00055.png}} \\
    \vspace{-0.9cm}
    \caption{\textbf{Editing on background atlases.} The source and edited background atlases are shown in the top row, and the resulting frames are in the same column. The background atlas can be treated as a natural panorama image for image editing. In addition, the edited background atlases can be directly used for the entire video since each visible pixel is edited in atlases.}
    \label{fig:supp_edit_bg_atlas}
\end{figure}
