# Supplementary material for: Shape-aware Text-driven Layered Video Editing
Source: arXiv:2301.13173 source file (2023-01-30)
Supplement: Supplementary file 3 [file fig_supp_edit_fg_atlas.tex]

\begin{figure}
    \centering
    \mpage{0.02}{\raisebox{2cm}{\rotatebox{90}{\hspace{1.8cm}Atlas}}}
    \frame{\includegraphics[width=0.23\linewidth]{figures/edit_atlas/fg_input/atlas.png}}
    \frame{\includegraphics[width=0.23\linewidth]{figures/edit_atlas/fg_example1/atlas.png}}
    \frame{\includegraphics[width=0.23\linewidth]{figures/edit_atlas/fg_example2/atlas.png}}
    \frame{\includegraphics[width=0.23\linewidth]{figures/edit_atlas/fg_example3/atlas.png}} \\
    \vspace{-2.1cm}
    \hline
    \vspace{0.1cm}
    \mpage{0.02}{\raisebox{2cm}{\rotatebox{90}{$\longleftarrow$ time}}}
    \frame{\includegraphics[width=0.23\linewidth]{figures/edit_atlas/fg_input/00025.png}}
    \frame{\includegraphics[width=0.23\linewidth]{figures/edit_atlas/fg_example1/00025.png}}
    \frame{\includegraphics[width=0.23\linewidth]{figures/edit_atlas/fg_example2/00025.png}}
    \frame{\includegraphics[width=0.23\linewidth]{figures/edit_atlas/fg_example3/00025.png}} \\
    \vspace{-1.5cm}
    \mpage{0.02}{\raisebox{2cm}{\rotatebox{90}{}}}
    \frame{\includegraphics[width=0.23\linewidth]{figures/edit_atlas/fg_input/00040.png}}
    \frame{\includegraphics[width=0.23\linewidth]{figures/edit_atlas/fg_example1/00040.png}}
    \frame{\includegraphics[width=0.23\linewidth]{figures/edit_atlas/fg_example2/00040.png}}
    \frame{\includegraphics[width=0.23\linewidth]{figures/edit_atlas/fg_example3/00040.png}} \\
    \vspace{-0.85cm}
    \mpage{0.02}{\raisebox{2cm}{\rotatebox{90}{}}}
    \frame{\includegraphics[width=0.23\linewidth]{figures/edit_atlas/fg_input/00055.png}}
    \frame{\includegraphics[width=0.23\linewidth]{figures/edit_atlas/fg_example1/00055.png}}
    \frame{\includegraphics[width=0.23\linewidth]{figures/edit_atlas/fg_example2/00055.png}}
    \frame{\includegraphics[width=0.23\linewidth]{figures/edit_atlas/fg_example3/00055.png}} \\
    \vspace{-0.9cm}
    \caption{\textbf{Editing on foreground atlases.} The source and edited foreground atlases are demonstrated in the top row, and the resulting frames are in the same column. The foreground atlas is an unwrapped texture due to the 3D object motion in the video. The distorted atlas poses a challenge for the general pre-trained Stable Diffusion to manipulate. As a result, the artifacts are shown in the rendered frames because of the incomplete and distorted edited atlases.}
    \label{fig:supp_edit_fg_atlas}
\end{figure}
