# Supplementary material for: Shape-aware Text-driven Layered Video Editing
Source: arXiv:2301.13173 source file (2023-01-30)
Supplement: Supplementary file 4 [file fig_supp_editing_image_and_atlas.tex]

\begin{figure*}
    \centering
    \mpage{0.02}{\raisebox{2cm}{\rotatebox{90}{\hspace{-0.3cm}Image}}}
    \frame{\includegraphics[width=0.22\linewidth]{figures/difference_editing/image_input.png}}
    \unskip\ \vrule height 1.9cm depth 2cm \ 
    \frame{\includegraphics[width=0.22\linewidth]{figures/difference_editing/image01.png}}
    \frame{\includegraphics[width=0.22\linewidth]{figures/difference_editing/image02.png}}
    \frame{\includegraphics[width=0.22\linewidth]{figures/difference_editing/image03.png}}\\
    \vspace{-2.05cm}
    \mpage{0.02}{\raisebox{2cm}{\rotatebox{90}{\hspace{1.4cm}FG atlas}}}
    \frame{\includegraphics[width=0.22\linewidth]{figures/difference_editing/atlas_input.png}}
    \unskip\ \vrule height 4cm depth 0.cm \ 
    \frame{\includegraphics[width=0.22\linewidth]{figures/difference_editing/atlas01.png}}
    \frame{\includegraphics[width=0.22\linewidth]{figures/difference_editing/atlas02.png}}
    \frame{\includegraphics[width=0.22\linewidth]{figures/difference_editing/atlas03.png}}\\
    \vspace{-2.4cm}
    \mpage{0.02}{\raisebox{2cm}{\rotatebox{90}{BG atlas}}}
    \frame{\includegraphics[width=0.22\linewidth]{figures/difference_editing/bg_input.png}}
    \unskip\ \vrule height 2.2cm depth 0.cm \ 
    \frame{\includegraphics[width=0.22\linewidth]{figures/difference_editing/bg02.png}}
    \frame{\includegraphics[width=0.22\linewidth]{figures/difference_editing/bg01.png}}
    \frame{\includegraphics[width=0.22\linewidth]{figures/difference_editing/bg03.png}}\\
    \vspace{-1.5cm}
    \caption{\textbf{Editing on foreground atlases.}}
    \label{fig:supp_editing_image_and_atlas}
\end{figure*}
