# Supplementary material for: Shape-aware Text-driven Layered Video Editing
Source: arXiv:2301.13173 source file (2023-01-30)
Supplement: Supplementary file 5 [file fig_supp_text2live_variant.tex]

\begin{figure*}
    \centering
    \mpage{0.02}{\raisebox{2cm}{\rotatebox{90}{Input}}}
    \frame{\includegraphics[width=0.22\linewidth]{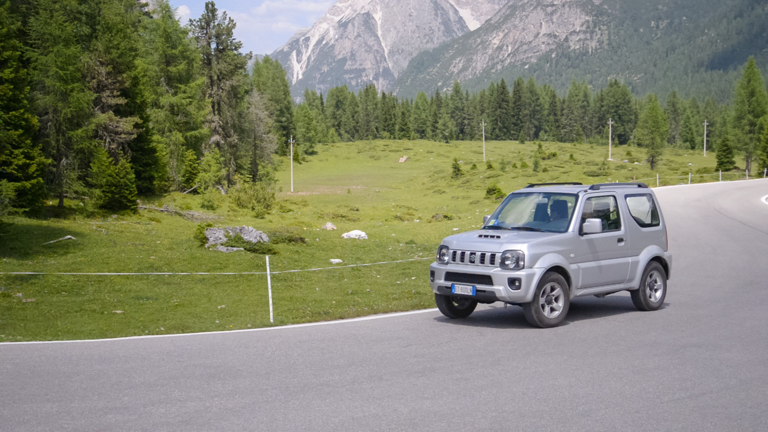}}
    \frame{\includegraphics[width=0.22\linewidth]{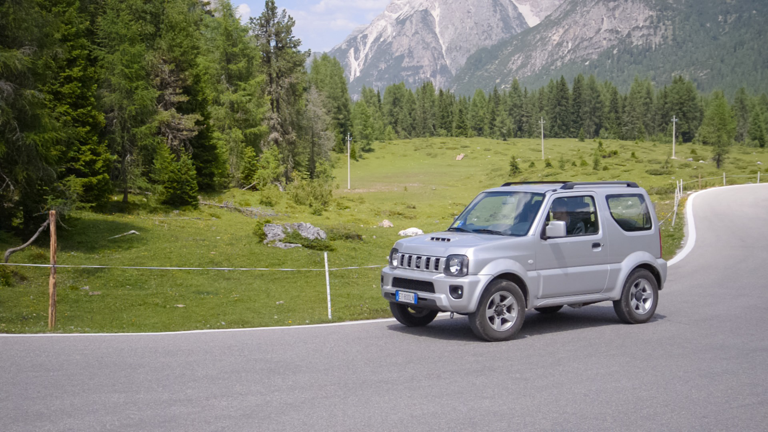}}
    \frame{\includegraphics[width=0.22\linewidth]{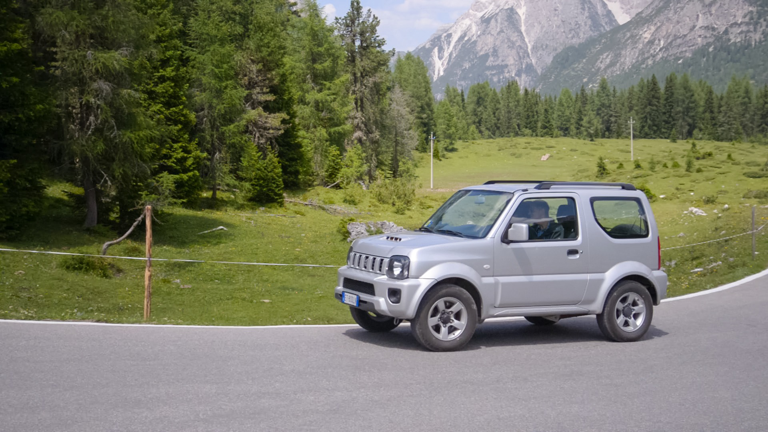}}
    \frame{\includegraphics[width=0.22\linewidth]{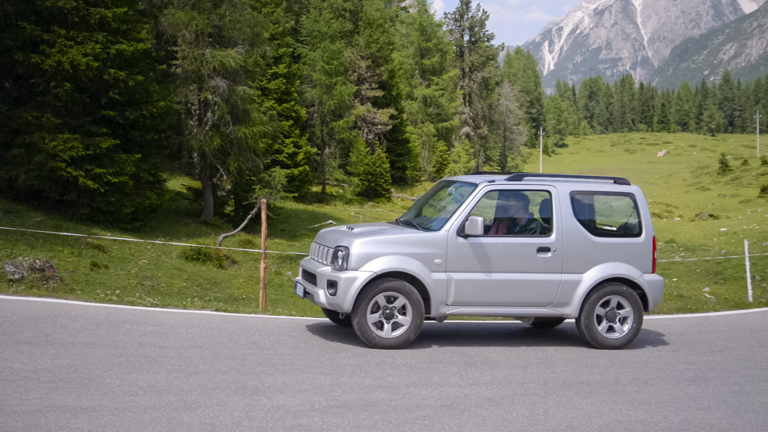}} \\
    \vspace{-1.175cm}
    \mpage{0.02}{\raisebox{2cm}{\rotatebox{90}{Ours}}}
    \frame{\includegraphics[width=0.22\linewidth]{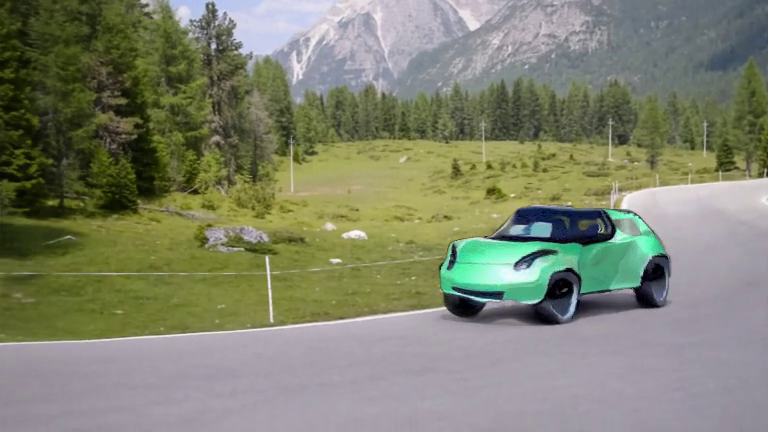}}
    \frame{\includegraphics[width=0.22\linewidth]{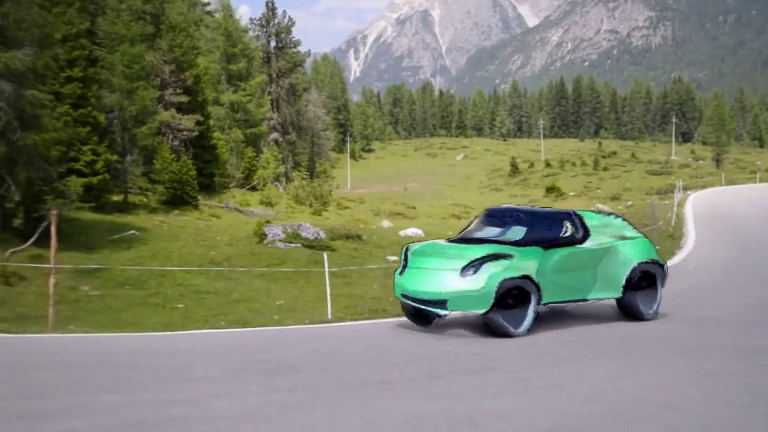}}
    \frame{\includegraphics[width=0.22\linewidth]{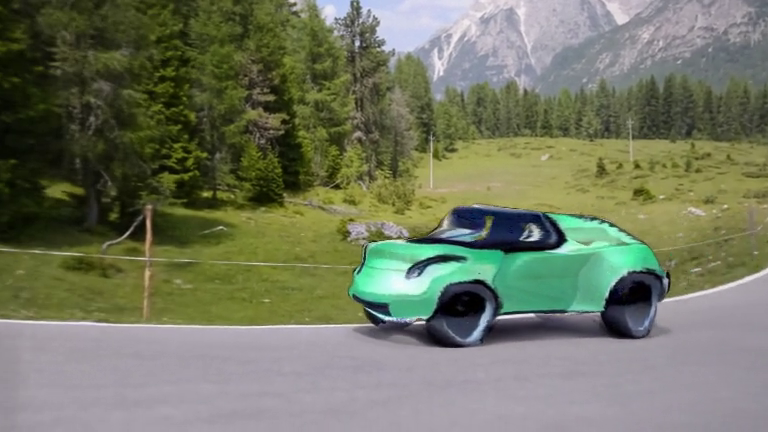}}
    \frame{\includegraphics[width=0.22\linewidth]{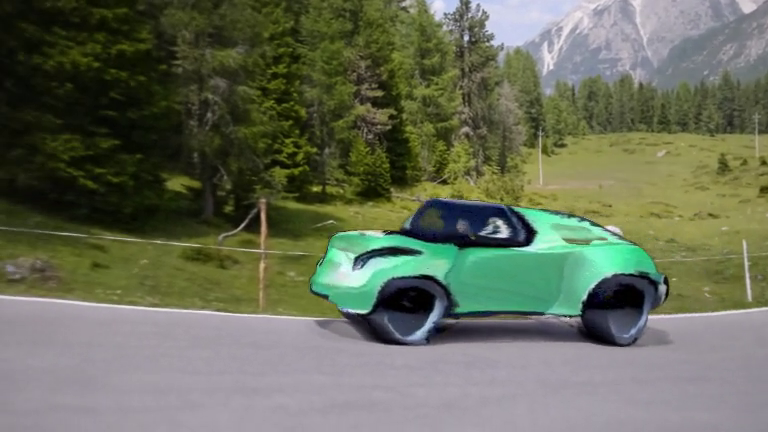}} \\
    \vspace{-1.15cm}
    \mpage{0.02}{\raisebox{2cm}{\rotatebox{90}{Text2LIVE~\cite{bar2022text2live}}}}
    \frame{\includegraphics[width=0.22\linewidth]{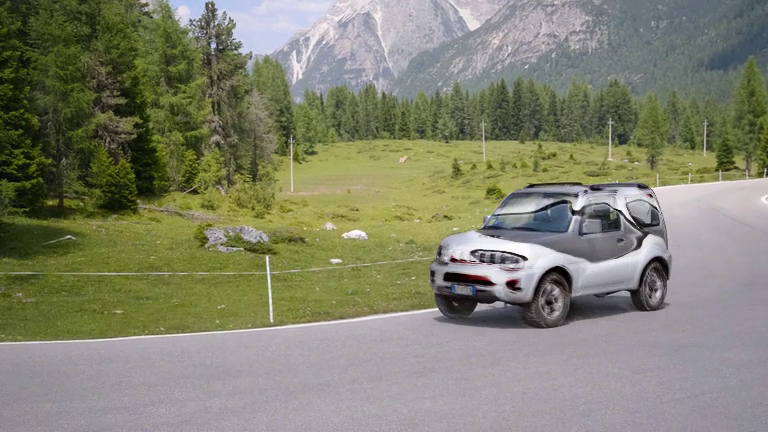}}
    \frame{\includegraphics[width=0.22\linewidth]{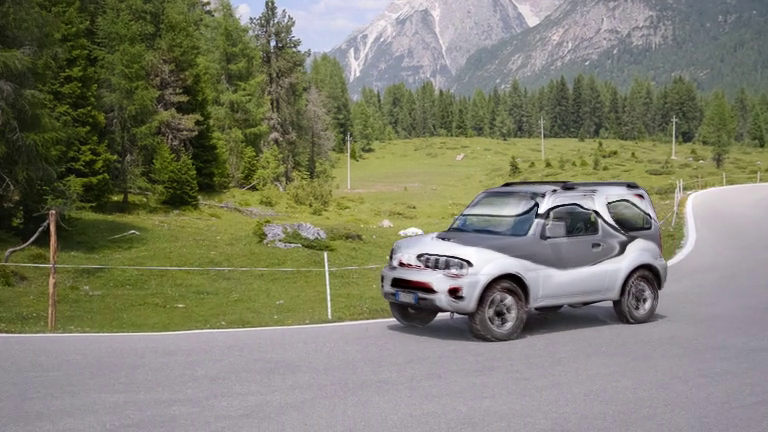}}
    \frame{\includegraphics[width=0.22\linewidth]{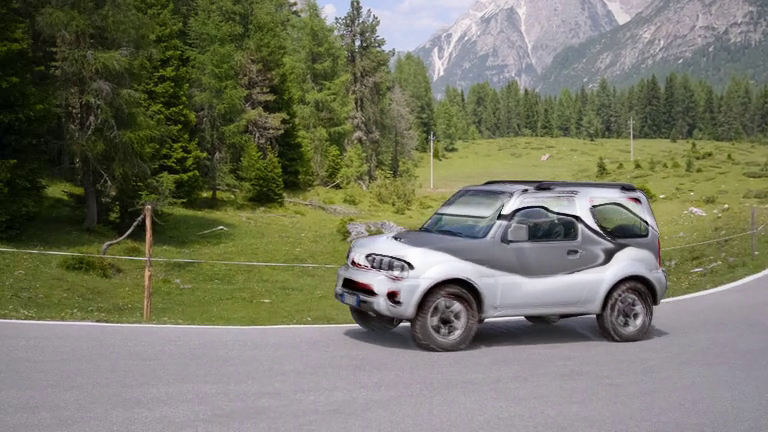}}
    \frame{\includegraphics[width=0.22\linewidth]{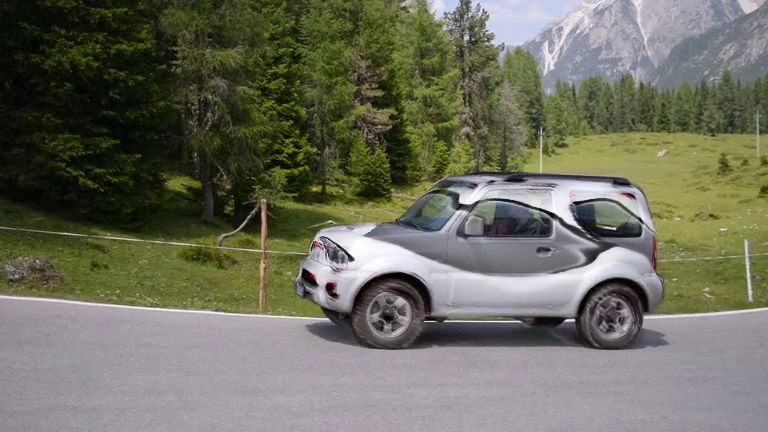}} \\
    \vspace{-1.85cm}
    \mpage{0.02}{\raisebox{2cm}{\rotatebox{90}{\small{\cite{bar2022text2live} w/o struct.}}}}
    \frame{\includegraphics[width=0.22\linewidth]{figures/visual_comparison/sports/text2live_wo_structure/00036.png}}
    \frame{\includegraphics[width=0.22\linewidth]{figures/visual_comparison/sports/text2live_wo_structure/00042.png}}
    \frame{\includegraphics[width=0.22\linewidth]{figures/visual_comparison/sports/text2live_wo_structure/00048.png}}
    \frame{\includegraphics[width=0.22\linewidth]{figures/visual_comparison/sports/text2live_wo_structure/00054.png}} \\
    \vspace{-1.825cm}
    \mpage{0.02}{\raisebox{2cm}{\rotatebox{90}{\small{\cite{bar2022text2live} w/ trained UV}}}}
    \frame{\includegraphics[width=0.22\linewidth]{figures/visual_comparison/sports/text2live_w_trained_uv/00036.png}}
    \frame{\includegraphics[width=0.22\linewidth]{figures/visual_comparison/sports/text2live_w_trained_uv/00042.png}}
    \frame{\includegraphics[width=0.22\linewidth]{figures/visual_comparison/sports/text2live_w_trained_uv/00048.png}}
    \frame{\includegraphics[width=0.22\linewidth]{figures/visual_comparison/sports/text2live_w_trained_uv/00054.png}} \\
    \vspace{-2.3cm}
    \caption{\textbf{Visual comparison with modified Text2LIVE~\cite{bar2022text2live}.} We attempt to modify the official Text2LIVE to enable shape-aware editing. We remove the shape preservation loss, but the results still remain in the source shape due to the fixed UV (as in the 4\textsuperscript{th} row, w/o struct.) Therefore, we further try to jointly train the per-frame UV maps during the optimization. However, the training of UV maps makes noisy and temporal flickering in the 5\textsuperscript{th} row, w/ trained UV). In sum, we believe that Text2LIVE is not feasible for shape-aware editing.}
    \label{fig:supp_text2live_variant}
\end{figure*}
