# Supplementary material for: Shape-aware Text-driven Layered Video Editing
Source: arXiv:2301.13173 source file (2023-01-30)
Supplement: Supplementary file 6 [file fig_supp_user_study.tex]

\begin{figure}
    \centering
    \includegraphics[width=\linewidth]{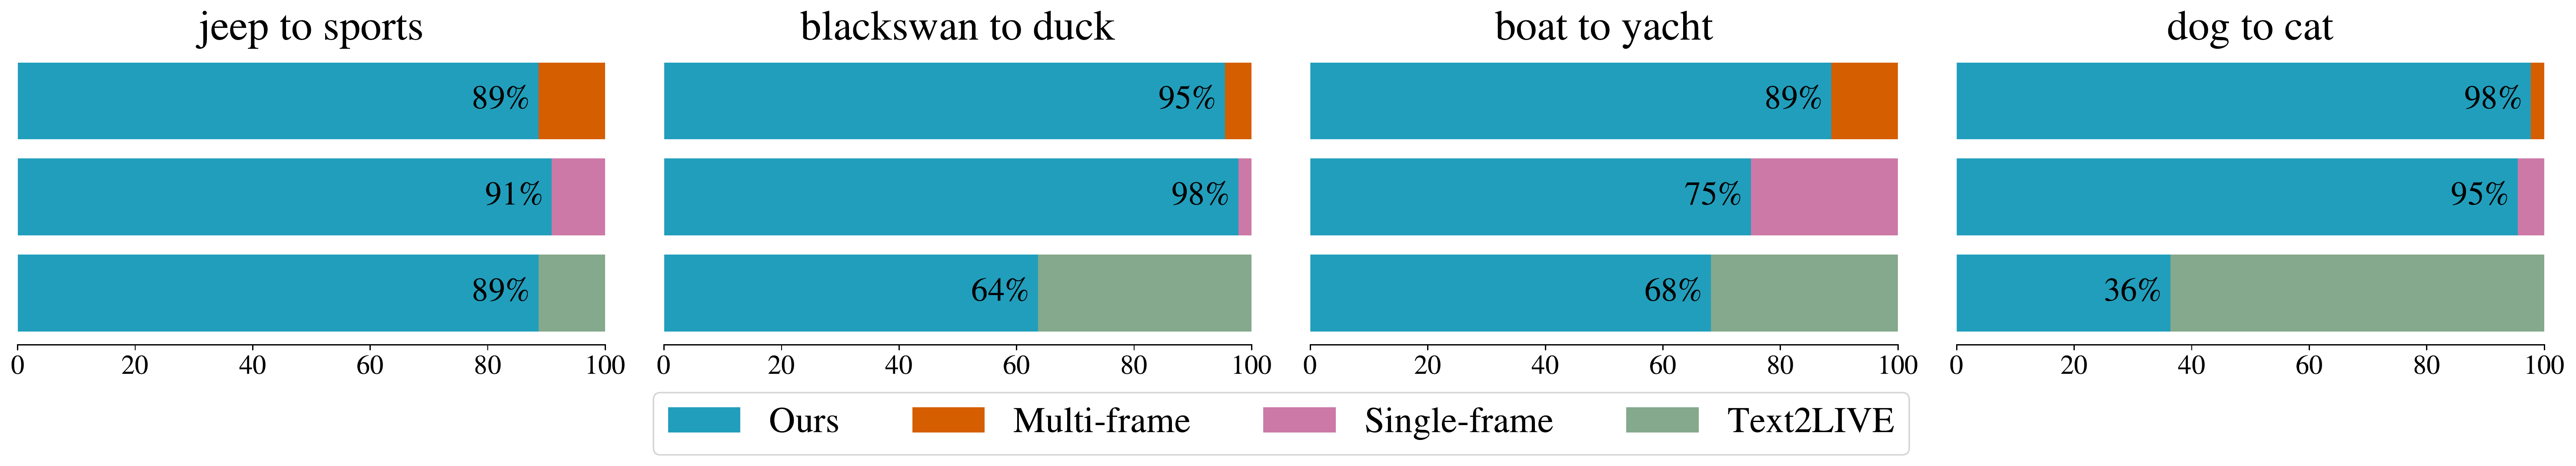}
    \caption{\textbf{Quantitative comparison by human evaluation.} We show the users' judgment of our method with each of compared baseline methods and Text2LIVE~\cite{bar2022text2live}. In general, most participants prefer our method to other approaches.}
    \label{fig:supp_user_study}
\end{figure}
